# Supplementary material for: Stroke-based Character Reconstruction
Source: arXiv:1806.08990 source file (2018-11-29)
Supplement: Supplementary file 1 [file appendix.tex]

\section{Appendix}
\subsection{Network structure}
The network structure diagram is shown in Figure~\ref{fig:visual}, Figure~\ref{fig:actor} and Figure~\ref{fig:critic}, where \texttt{FC} refers to a fully-connected layer, \texttt{Conv} is a convolution layer and \texttt{Pooling} is a $2\times2$ max pooling. Only the first convolution kernel is $7\times7$, the rest are $3\times3$. The numbers of convolution filter are 16, 32, 32, 64, 128, 128 respectively. All Leaky ReLU activations between the layers have been omitted for brevity. The activation function after actor and critic network is a linear function. The output of the actor network are clipped into range [0,1].
\begin{figure}[ht]
\centering
\input{architecture/visual.tex}
\caption{The architecture of the \textbf{visual network}. }
\label{fig:visual}
\end{figure}
\begin{figure}[ht]
\centering
\input{architecture/actor.tex}
\caption{The architecture of the \textbf{actor network}. }
\label{fig:actor}
\end{figure}
\begin{figure}[ht]
\centering
\input{architecture/critic.tex}
\caption{The architecture of the \textbf{critic network}.}
\label{fig:critic}
\end{figure}
